# Supplementary material for: Strain pattern in supercooled liquids
Source: arXiv:1606.03353 ancillary file (2016-08-05)
Supplement: Supplementary file 1 [file Illing_etal_2016_supp_mat.pdf]

## Supplemental Information for: Strain pattern in supercooled liquids

Bernd Illing,[1] Sebastian Fritschi,[1] David Hajnal,[2] Christian Klix,[1] Peter Keim,[1] and Matthias Fuchs[1]

[1] *University of Konstanz, D-78457 Konstanz, Germany*

[2] *Johannes Gutenberg-University Mainz, D-55099 Mainz, Germany*

*Present Adress: BASF SE, Carl-Bosch-Strasse 38, D-67056 Ludwigshafen, Germany*

(Dated: August 3, 2016)

The supplemental material contains experimental details, information on the simulation and coarse-graining methods, as well as theoretical and numerical details.

### EXPERIMENTAL ASPECTS

Video microscopy provides access to the full phase space information of the colloidal monolayer at all relevant time and length scales. We record the trajectories of about 2300 colloidal particles (the whole system consists of more than $10^5$ particles) confined to two dimensions by sedimentation at a flat water-air interface. This interface is realized by a water droplet hanging by surface tension in a top-sealed cylindrical hole (6 mm in diameter) of a glass cuvette. The volume and thus the curvature of the droplet is actively regulated by several computer controlled regulation loops to be completely flat for a duration of several months providing excellent long time stability. The species A (diameter $\sigma = 4.5\,\mu m$) and B ($\sigma = 2.8\,\mu m$) have a relative concentration of $\xi = N_B/(N_A + N_B) \approx 50\,\%$ where $N_A$ and $N_B$ are the number of particles of both species in the field of view. The binary mixture prevents the system from crystallization. The ratio of the repulsive potential energy versus thermal energy (causing Brownian motion) can be controlled *in situ* by an external magnetic field $H$ due to the superparamagnetic nature of the particles. It is expressed by the dimensionless system parameter

$$\Gamma = \frac{\mu_0}{4\pi} \cdot \frac{H^2 \cdot (\pi n)^{3/2}}{k_B T}(\xi \cdot \chi_B + (1-\xi)\cdot \chi_A)^2\,, \qquad (4)$$

which effectively acts as an inverse temperature or, since particle number and volume are fixed, can be interpreted as a dimensionless pressure. Here, $n$ denotes the area density and is computed via a Voronoi tessellation. $\chi_{A,B}$ represent the susceptibilities of species A and B, respectively. After equilibration at low $\Gamma$, the system was cooled down stepwise. With a frame rate of $\approx 0.5\,\mathrm{s}^{-1}$, sampling times of $2 \times 10^4$ seconds for the fluid system and $1.2 \times 10^5$ s for the glassy system were achieved. As the intrinsic time equals $1/(nD_0) \approx 1.5 \times 10^3$ seconds, this is sufficiently long to probe dynamics up to the relaxation time regime. Additional details of the setup and the active regulation of the interface are described in [25].

The structural relaxation times used in the main text, are estimated by fitting an exponential decay to the density-correlation functions $\Phi_q(t)$ as shown in Fig. 4.

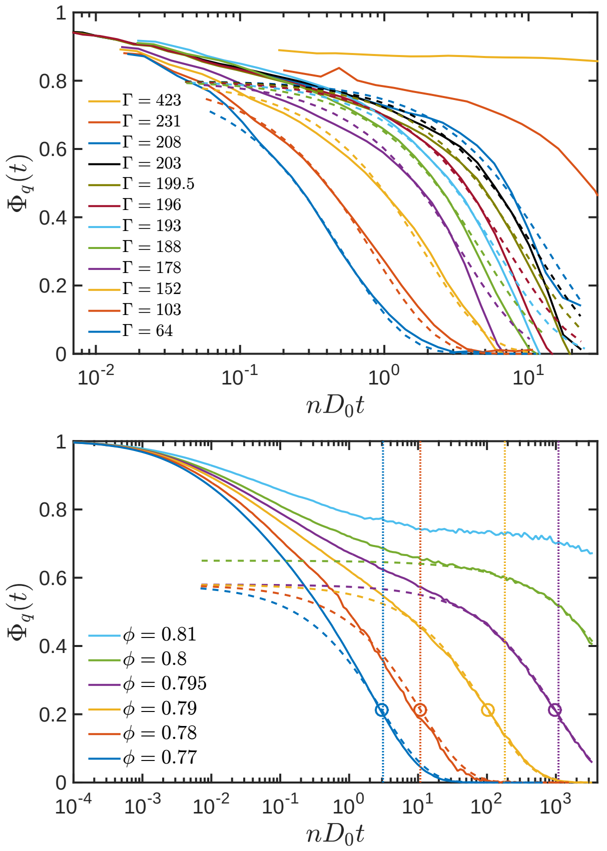


FIG. 4: Experimental (top) and simulational (bottom) incoherent density correlation data for different $\Gamma$ and $\phi$ (see legends) for wavevectors $qa = 7.3$ (experiment) and $qa = 7.4$ (simulation) (corresponding to the first peak of the structure factor $S(q)$). The dashed lines show stretched-exponential fits $\Phi_q(t) = A\exp(-(t/\tau)^\beta)$ with $A = 0.80$, $\beta = 1.0$ (exp.) and $A = 0.58$, $\beta = 0.65$ (sim., $\phi < 0.8$). For the simulational data, the fitted $\tau$ is marked by circles and, additionally, $\tau_\eta = const. \cdot \eta/\mu_c$ is indicated by dotted vertical lines, with shear modulus $\mu_c = \mu(\phi_c) = 48.8\, nk_BT$ and shift factor $const. = 4.6$.

### SIMULATIONAL ASPECTS

We perform simulations on a 2D binary mixture of hard disks undergoing Brownian motion employing an event-driven simulation algorithm [35, 36]. The system contains $N = 16000$ particles, is made up of a 50:50 mix-

ture with diameters $d_A = 1$, $d_B = 1.4$, and is equilibrated by Newtonian dynamics before data are collected. The packing fraction, giving the ratio of the area occupied by the disks to the area of the system, varies from $\phi = 0.77$ to $\phi = 0.81$, hence close to the mode-coupling glass transition point $\phi_c \approx 0.795$ [32]. The shown strain correlation data is based on at least 150 independent single runs for each packing fraction. The elastic moduli $\mu$ and $\mu^{\|}$ are determined from particle trajectories as described in [20], the shear viscosity $\eta$ is calculated via momentum transfer at collisions as in [36, 37]. The structural relaxation time is estimated by fitting a stretched exponential decay to the density-correlation function as shown in Figure 4.

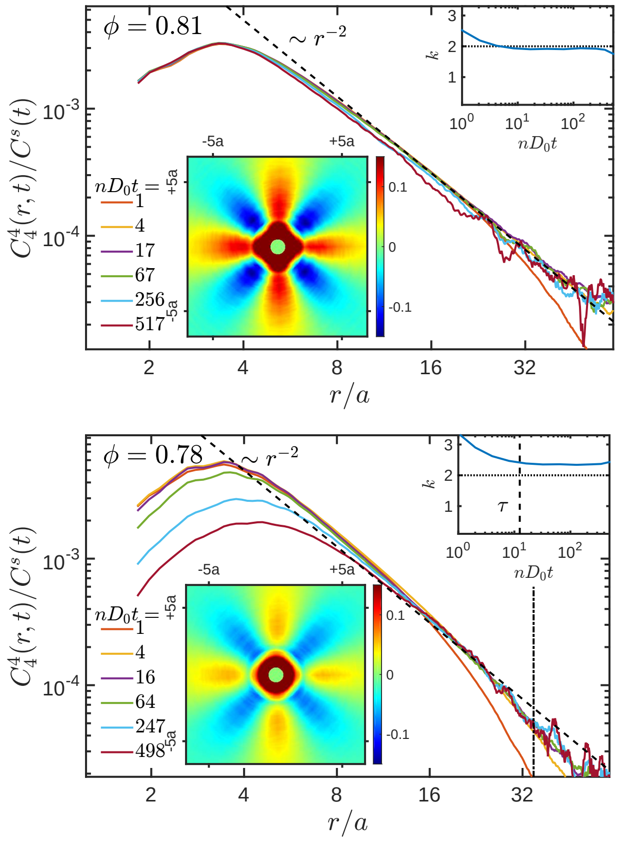


FIG. 5: Rescaled mean-squared strain data from BD simulations of a binary hard disk mixture in a glass (upper panel; $\phi = 0.81$) and a fluid (lower panel; $\phi = 0.78$) state at different times (see legend). The spherical harmonic strain correlation functions $C_4^4(r,t)/C^s(t)$ are rescaled to overlap in the far-field power law decay. Main panels show the $1/r^k$-power law decay (dashed black) valid up to $r = \mathcal{O}(L)$ (a vertical black dash-dotted line indicates $r = \pi L$), with exponent (upper insets) $k = 2$ varying little with time. The contourplots (lower insets) of the long-time limit of $C_{xy}(\mathbf{r},t)/C_{xy}(\mathbf{r}=0,t)$ illustrate the corresponding $\cos(4\theta)$-symmetry at $nD_0t = 256$ (upper panel) and $nD_0t = 247$ (lower panel), respectively.

## COARSE GRAINING METHOD

To obtain smooth strain fields from discrete particle positions, a coarse graining approach following [22] is applied. Single particle displacements are obtained from differences of particle positions, $\mathbf{u}_i(\mathbf{r}_i,t',t) = \mathbf{r}_i(t') - \mathbf{r}_i(t'-t)$, and then coarse-grained:

$$\mathbf{u}(\mathbf{r},t',t) = \frac{1}{\varrho(\mathbf{r},t')}\sum_{i=1}^{N}\mathbf{u}(\mathbf{r},t',t)\phi(|\mathbf{r}-\mathbf{r}_i(t')|,r_c), \quad (5)$$

where $\varrho(\mathbf{r},t')$ is the corresponding coarse-grained density. Running averages over $t'$ are used to smoothen the data. Considering the radial symmetry of the collective mean squared strain function (CMSS) $C_{xy}(\mathbf{r},t)$, the analysis is implemented in polar coordinates using a Gaussian coarse graining function:

$$\phi(r,r_c) = \frac{1}{D_g(r_c,\sigma)}\begin{cases}\exp\left(-\frac{r^2}{2\sigma^2}\right) & \text{if } r < r_c\\ 0 & \text{else}\end{cases} \quad (6)$$

with normalization $D_g(r_c,\sigma) = 2\pi\sigma^2\left(1-\exp\left(-\frac{r_c^2}{2\sigma^2}\right)\right)$. Various cut-off radii $r_c$ were tested for consistency and $r_c/a = 2$ was found to be best, since it captures all three (binary mixture) first-order but no second-order peaks of the radial pair distribution function. Also the coarse graining function used by Ref. [1] and a cartesian grid was tested which gave consistent results (not shown) for the CMSS in the far field ($r/a \gg 1$) relevant for the above analysis. We also integrated up the coarse-grained velocity field instead of using Eq. (5) as done in Ref. [1], and found only small quantitative differences.

From the coarse-grained displacement field described above the strain is obtained by differentiation [22]. The normalized spatial shear CMSS

$$\tilde{C}_{xy}(\mathbf{r},t) = \frac{C_{xy}(\mathbf{r},t)}{C_{xy}(\mathbf{r}=0,t)} \quad (7)$$

is sampled for experimental and simulational data, and shown in the contour plots in Figs. 1 (main text, experiment) and 5 (simulation). We tested that using the non-linearized form of the strain tensor gives quantitative but not qualitative differences to the observed Eshelby-pattern in liquid states for up to the times considered. The far-field power-law was fitted in the range $r/a \in [5,12]$ ($r/a \in [9,17]$ at $\Gamma = 423$) for experimental data and $r/a \in [10,22]$ for simulational data. The projection on $\cos(4\theta)$ gives by comparison with Eq. (1)

$$\frac{1}{\pi}\int_0^{2\pi} d\theta \cos(4\theta)\tilde{C}_{xy}(\mathbf{r},t) \to \underbrace{\frac{1}{C_{xy}(\mathbf{r}=0,t)}}_{b}\frac{C^s(t)}{4\pi n r^2} \quad (8)$$

and with this the relation: $C^s(t) = b \cdot C_{xy}(\mathbf{r}=0,t)$. The parameter $b$ is determined by fitting a $1/r^2$-law to

the long distance (same range as above) part of this projection and was found to be constant over time for each temperature.

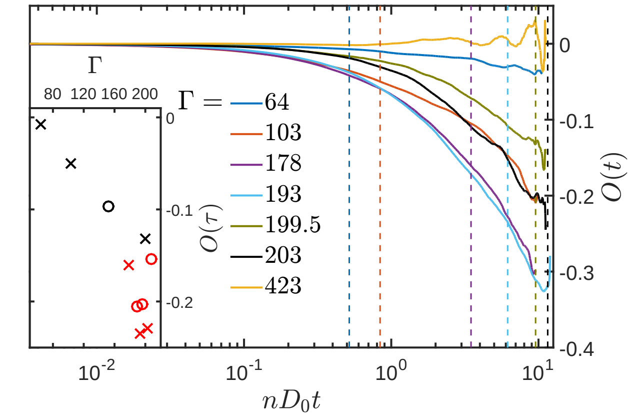


FIG. 6: The global averaged strain $O(t)$ as a function of time for selected temperatures. While the glass data do not show a significant global strain, some of the fluid data do. The inset shows $O(t = \tau)$ for fluid states at the $\alpha$-relaxation time $\tau$ (vertical dashed lines); crosses (circles) are used for the data (not) shown in the main panel. Data in the fluid state showing isotropic offsets in the CMSS $C_{xy}(\mathbf{r}, t)$ (red symbols in inset) tend to exhibit larger global strain due to experimental perturbations as the ones without offsets (black symbols).

From an experimental point of view, extreme care has to be taken to stabilize the monolayer in the liquid state ($\Gamma < \Gamma_g$) in hanging droplet geometry. Some data in the liquid state show, in addition to the above discussed Eshelby-patterns, nearly isotropic offsets in the CMSS $C_{xy}(\mathbf{r}, t)$, which are absent in the simulations. They are assumed to stem from macroscopic shears (i.e. on length-scales larger than the field of view) due to experimental perturbations. To independently detect these states, we investigated the averaged global strain $O(t)$, normalized by its variance as function of time for various temperatures,

$$O(t) = \frac{\langle \varepsilon_{xy}(\mathbf{r}, t)\rangle_{\mathbf{r}}}{\sqrt{\langle \varepsilon_{xy}^2(\mathbf{r}, t)\rangle_{\mathbf{r}}}}, \tag{9}$$

where averaging was done over space $\mathbf{r}$, as indicated, and over different time windows to increase statistics. Figure 6 shows the time evolution of $O(t)$ for several $\Gamma$ (only selected ones are shown, not to overcrowd the main figure). To compare different temperatures, we take the global strain at the $\alpha$-relaxation time, $O(t = \tau)$ with $\tau$ indicated by vertical dashed lines in Fig. 6, and plot this in the inset (all fluid $\Gamma$ included). Data sets where isotropic offsets in the CMSS were noticed (red symbols) exhibit large (negative) values for $O(t = \tau)$ supporting the assumption that they originate from global strain in the colloidal layer. However, the Eshelby-pattern could still be observed and the analysis of the spatial power law decay performed, because the isotropic offsets are eliminated in the projection to $C_4^4$.

## BEYOND THE INCOMPRESSIBILITY APPROXIMATION

It is straightforward to calculate the transversal collective mean-squared strains in compressible isotropic systems from the Fourier-transformed displacement fluctuations. This requires, besides the transversal collective mean-squared displacement $C_q^{\perp}(t)$, also the longitudinal one, denoted $C_q^{\parallel}(t)$:

$$C_{xy}(\mathbf{r}, t) = \int \frac{d^d\mathbf{q}}{(2\pi)^d}\, e^{-i\mathbf{q}\cdot\mathbf{r}} \tag{10}$$
$$\left[\left(C^{\perp}(q,t) - C^{\parallel}(q,t)\right)\frac{-q_x^2 q_y^2}{q^2} + C^{\perp}(q,t)\,\frac{q_x^2 + q_y^2}{4}\right] \;,$$

Starting from Ref. [20], the generalized hydrodynamics approximation leads to a concise relation for the longitudinal mean-squared displacements using a temporal Laplace transformation, $C(s) = \int_0^\infty dt e^{-st} C(t)$:

$$C_{gH}^{\parallel}(q, s) = \frac{2D_0/s}{s + \frac{q^2 D_0}{k_B T n}\left(\frac{1}{\kappa^T} + sG^{\parallel}(s)\right)}\;. \tag{11}$$

It contains the generalized frequency-dependent longitudinal stress modulus, $G^{\parallel}(s) = G^{\mathrm{B}}(s) + (2 - 2/d)G^{\perp}(s)$ in $d$ dimensions, where the shear modulus was defined in the main text and the bulk modulus is given by [27]: $G^{\mathrm{B}}(t) = \frac{n}{k_B T}\,\langle \sigma^{\mathrm{B}}(t_{\mathcal{Q}})^*\, \sigma^{\mathrm{B}}\rangle$ with $\sigma^{\mathrm{B}} = \frac{1}{d}\sum_\alpha \sigma_{\alpha\alpha} + p$ and pressure $p$.

| Simulation | | | Experiment | | |
|---|---|---|---|---|---|
| $\phi$ | $\frac{\mu}{nk_BT}$ | $\frac{\mu^{\parallel}}{nk_BT}$ | $\Gamma$ | $\frac{\mu}{nk_BT}$ | $\frac{\mu^{\parallel}}{nk_BT}$ |
| 0.795 | 48.8 | 355.2 | | | |
| 0.8 | 59.9 | 424.1 | 188 | 14 | 37 |
| 0.805 | 72.6 | 505.6 | 193 | 18 | 36 |
| 0.81 | 90.4 | 618.7 | 196 | 20 | 49 |
| Theory (MCT) | | | 208 | 31 | 129 |
| $\Gamma$ | $\frac{\mu}{nk_BT}$ | $\frac{\mu^{\parallel}}{nk_BT}$ | 231 | 42 | 182 |
| 107 | 0 | 4.8 | 423 | 99 | 403 |
| 114 | 0 | 4.8 | | | |
| 118 | 21.9 | 52.7 | | | |

TABLE I: Transversal $\mu$ and longitudinal $\mu^{\parallel}$ modulus from simulation, theory (MCT) and experiment.

Clearly, longitudinal displacement fluctuations stay bounded for all times (see also Fig. 7, top panel):

$$C_{gH}^{\parallel}(q, t) \le C_{gH}^{\parallel}(q, t \to \infty) = \frac{2k_B T n\kappa^T}{q^2}\;. \tag{12}$$

The approximation of an incompressible dispersion sets $\kappa^T = 0$ and thus neglects longitudinal displacements.

The corrections to the asymptotic limits in Eq. (3) can now be obtained. In fluid states, the finite longitudinal displacements become negligible for long times, and $C^s(t \to \infty) \to \frac{2k_BTn}{\eta} t$ remains valid. In glass states, $C^s(t \to \infty) = 2k_BTn \left(1/\mu - 1/\mu^{\parallel}\right)$ follows with longitudinal modulus $\mu^{\parallel} = G^{\parallel}(t \to \infty) + \frac{1}{\kappa_T}$. To evaluate the error of the incompressibility assumption, table I contains the glass moduli of the considered systems.

## MODE COUPLING APPROXIMATION

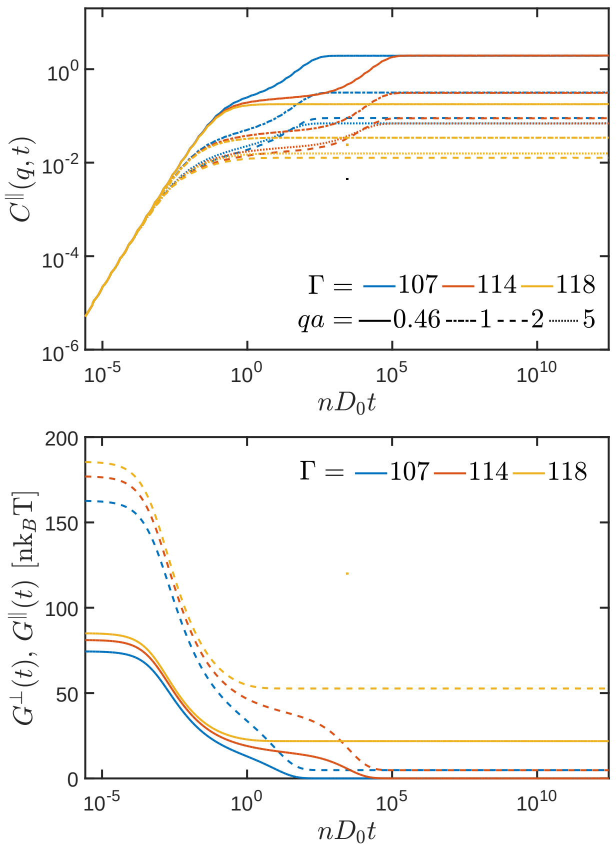


FIG. 7: Top: Numerical results for the longitudinal collective mean-squared displacement $C^{\parallel}(q,t)$ from MCT for various wavevectors $q$ and values for $\Gamma$ in the fluid and the glass state. Bottom: Numerical results for the long wavelength limit of the longitudinal (dashed) and transversal (solid) memory kernel $G^{\parallel}(q,t)$, $G^{\perp}(q,t)$ respectively.

Performing the standard MCT approximation [40], the stress kernels take the explicit form (in $d$ dimensions, for monodisperse particles):

$$\mathbf{G}(\mathbf{q},t) = \frac{n^2}{2k_BT}\int \frac{d^dk}{(2\pi)^d}\frac{1}{q^2}\left[\mathbf{k}c_k + (\mathbf{q}-\mathbf{k})c_{|\mathbf{k}-\mathbf{q}|}\right] \left[\mathbf{k}c_k + (\mathbf{q}-\mathbf{k})c_{|\mathbf{k}-\mathbf{q}|}\right] S_k S_{|\mathbf{k}-\mathbf{q}|}\Phi_k(t)\Phi_{|\mathbf{k}-\mathbf{q}|}(t)\ , \quad (13)$$

where $\Phi_q(t) = \langle \delta\varrho^*_{\mathbf{q}}(t)\delta\varrho_{\mathbf{q}}\rangle / S_q$ is the normalized density correlator and $c_k$ the direct correlation function ($S_k = 1/(1-nc_k)$). It connects to the (longitudinal) memory function of the equations of motion for density correlators $m_q(t) = \frac{k_BT}{n}\mathbf{q}\cdot\mathbf{G}(\mathbf{q},t)\cdot\mathbf{q}/q^2$. The limit of $q \to 0$ gives the familiar MCT expression for the macroscopic moduli [40]:

$$G^{\parallel}(t) = \frac{n^2}{2k_BT}\int \frac{d^dk}{(2\pi)^d}\left(c_k + \frac{(\mathbf{k}\cdot\mathbf{q})^2}{kq^2}c'_k\right)^2 S_k^2\Phi_k^2(t)\ ,$$

and

$$G^{\perp}(t) = \frac{n^2}{2k_BT}\int \frac{d^dk}{(2\pi)^d}k_x^2k_y^2\,(\frac{1}{k}c'_kS_k\Phi_k(t))^2\ .$$

## NUMERICAL DETAILS

Based on the numerical solutions of the MCT equations [32] and Eqs. (2,13) both, the longitudinal $C^{\parallel}(q,t)$ and the transversal part $C^{\perp}(q,t)$ of the mean-squared displacement correlator were calculated. Whereas the latter was already shown (Fig. 2) and discussed in the main text, the former is shown in Fig. 7, top panel, to confirm that the longitudinal component stays bounded at all times. $\mathbf{G}(\mathbf{q},t)$ was calculated for two fluid states $\Gamma = 107, 114$ and one glass state $\Gamma = 118$ with the mode-coupling glass transition at $\Gamma_c = 115$. The resulting long wavelength limit of the tranversal $G^{\perp}(q,t)$ and longitudinal $G^{\parallel}(q,t)$ part of the memory kernel is shown in Fig. 7, bottom panel. Here, the integrals over wavevectors $q$ and time $t$ are discretized to sums using a linear 250-node grid for $q$ and a semi-logarithmic grid for $t$. The limit of small $q$ is realized by choosing the smallest $q$-vector $qa = 0.4606$ (see inset of Fig. 2, main text). The time grid consists of 60 blocks containing 128 equally spaced time steps doubling from one block to the next one, creating a grid spanning over 15 decades in time.

### References


[35] A. Scala, T. Voigtmann, and C. De Michele, J. Chem. Phys. **126**, 134109 (2007).
[36] O. Henrich, F. Weysser, M. E. Cates, and M. Fuchs, Philos. Trans. R. Soc. A **367**, 5033 (2009).
[37] B. J. Alder, D. M. Gass, and T. E. Wainwright, J. Chem. Phys. **53**, 3813 (1970).
